# Supplementary material for: Proposed Rabi-Kondo Correlated State in a Laser-Driven Semiconductor Quantum Dot
Source: arXiv:1211.6837 source file (2013-10-11)
Supplement: Supplementary file 1 [file SupplementalMaterial_Proposed_Rabi-Kondo_Correlated_State_in_a_Laser-Driven_Semiconductor_Quantum_Dot.pdf]

## Supplemental Material: "Proposed Rabi-Kondo Correlated State in a Laser-Driven Semiconductor Quantum Dot"

### Discussion of the Hamiltonian $H$ and Born-Markov approximation

Here we discuss the form of the Rabi-Kondo model Hamiltonian $H$, Eq. (1) in the main text, in more detail. The QD part reads $H_{\mathrm{QD}} = \sum_\sigma (\varepsilon_\mathrm{e} - U_{\mathrm{eh}} n_\mathrm{h}) n_{\mathrm{e}\sigma} + U n_{\mathrm{e}\uparrow} n_{\mathrm{e}\downarrow} + \varepsilon_\mathrm{h} n_\mathrm{h}$. The eigenenergies are conveniently displayed vs. the gate voltage which controls $\varepsilon_\mathrm{e}$ and $\varepsilon_\mathrm{h}$, in Fig. S1(a). The lowest energy QD state in the subspace with hole number $n_\mathrm{h} = 0$ or 1 is denoted by a purple or blue solid line, respectively. We focus on a gate voltage regime around $V_0$, as marked in Fig. S1(a). In this regime the lowest energy QD states carry one negative charge. Applying a monochromatic laser with photon energy $\omega_\mathrm{L} \simeq \varepsilon_\mathrm{h}$ leads to the rotating frame Hamiltonian $H_{\mathrm{QD,L}} = \sum_\sigma (\varepsilon_\mathrm{e} - U_{\mathrm{eh}} n_\mathrm{h}) n_{\mathrm{e}\sigma} + U n_{\mathrm{e}\uparrow} n_{\mathrm{e}\downarrow} + (\varepsilon_\mathrm{h} - \omega_\mathrm{L}) n_\mathrm{h}$, effectively shifting the purple line to the vicinity of the blue line. If the detuning $\delta_\mathrm{L}$ to the bare QD transition is small, then there exists a low energy description of $H_{\mathrm{QD,L}}$ involving only the states $|\uparrow\rangle, |\downarrow\rangle$ and the trion $|\uparrow\downarrow\Uparrow\rangle$ shown in Fig. 1(a) of the main text.

We now add to $H_{\mathrm{QD,L}}$ the QD-laser coupling in rotating wave approximation, $H_{\mathrm{QD-L}} = \Omega e_\downarrow^\dagger h^\dagger + \mathrm{h.c.}$, (we assume a circularly polarized laser and apply optical selection rules to simplify the problem, see main text) and a radiative reservoir $H_{\mathrm{rad}}$ (leading to a spontaneous emission rate $\gamma_{\mathrm{SE}}$ on the order of $1\mu eV$). For $\Omega \gg \gamma_{\mathrm{SE}}$ a three-peak Mollow triplet, similar to the red curve in Fig. S1(b), can be detected in the RF spectrum. The central peak appears at the laser frequency, $\omega = \omega_\mathrm{L}$ and the two side peaks at detuning $\nu = \omega - \omega_\mathrm{L} = \pm 2\Omega$.

If we now include the fermionic bath (FB), $H_{\mathrm{FB}} = \sum_{k\sigma} \varepsilon_{k\sigma} c_{k\sigma}^\dagger c_{k\sigma}$, and the QD-FB hybridization $H_{\mathrm{QD-FB}}$, the Hamiltonian reads $H + H_{\mathrm{rad}}$ with $H$ as in Eq. (1) of the main text. For a weak QD-FB coupling and temperatures $T > T_\mathrm{K}$ we make a Born-Markov approximation for the QD-FB coupling [1, 2], the corresponding transition rates in the dressed-QD Master equation crucially rely on the ratio between laser Rabi frequency $\Omega$ and sample temperature $T$. While $\Omega \ll T$ leads to a broadening of the ordinary Mollow RF-spectrum by symmetric thermal rates $\gamma_\mathrm{T}$ in each dressed-state manifold, a dominant laser $\Omega \gg T$ results in asymmetric intra-manifold rates $\gamma_\Omega$ and an asymmetric doublet in the RF spectrum, see Fig. S1(b), along with the dressed-state schematics. In this case, the FB cannot provide the energy difference for an upward transition between the dressed states. In experiment, the formation of an asymmetric doublet would have to be carefully distinguished from the effect of a finite laser detuning [which we have set to zero in Fig. S1(b)].

To access Kondo physics, $T < T_\mathrm{K}$ is required and the Born-Markov treatment of the dressed QD-FB interaction is no longer valid. With the spectral function defined as

$$S(\nu) = \frac{1}{2\pi} \int_{-\infty}^{\infty} d\tau \left\langle (he_\downarrow)^\dagger (\tau) (he_\downarrow) \right\rangle_{\mathrm{ss}} e^{-i\nu\tau}. \tag{S1}$$

the RF-spectrum is given by $\gamma_{\mathrm{SE}} \cdot S(\nu)$ [3]. Here, the occurrence of $\gamma_{\mathrm{SE}}$ shows that $H_{\mathrm{rad}}$ has explicitly been used in the derivation. If the coupling to the radiative reservoir is weak (i.e. $\gamma_{\mathrm{SE}}$ smaller than all other energy scales), we neglect $H_{\mathrm{rad}}$ to higher order in Eq. (S1), i.e. we approximate $(he_\downarrow)^\dagger(\tau) \simeq e^{i\tau H}(he_\downarrow)^\dagger e^{-i\tau H}$. Further, a similar approximation is done for the steady state density matrix $\rho_{\mathrm{ss}}$ used in

Eq. (S1) ($\langle ... \rangle_{ss}$ denotes a trace over $\rho_{ss}$): We assume that thermalization of the system due to the solid state environment at temperature $T$ takes place on timescales much faster than spontaneous emission. Then, we neglect $H_{rad}$ for $\rho_{ss}$ and assert that

$$\rho_{ss} = \rho_{eq} = e^{-H/T}/\mathrm{Tr}\left(e^{-H/T}\right) \tag{S2}$$

serves as a good approximation of the steady state. This leads to a RF spectrum that has support for $\nu \lesssim T$ only. We will further discuss effects related to the neglect of $H_{rad}$ in the last section of this Supplemental Material.

With these two important simplifications, the numerical study is facilitated considerably, Eq. (S1) can be written in Lehmann form and we arrive at Eq. (2) of the main text where the eigenstates and -energies of $H$ (as computed approximately by NRG) are used.

To conclude, the main text investigates how the asymmetric two peak structure (blue line in Fig. S1(b) for $\Omega \gg T > T_K$) changes when we increase the QD-FB coupling beyond perturbatively weak values, i.e. increase $T_K$ above $T$. We investigate the more interesting regime $T_K \gg \Omega$ in detail and comment briefly on the case $T_K \ll \Omega$.

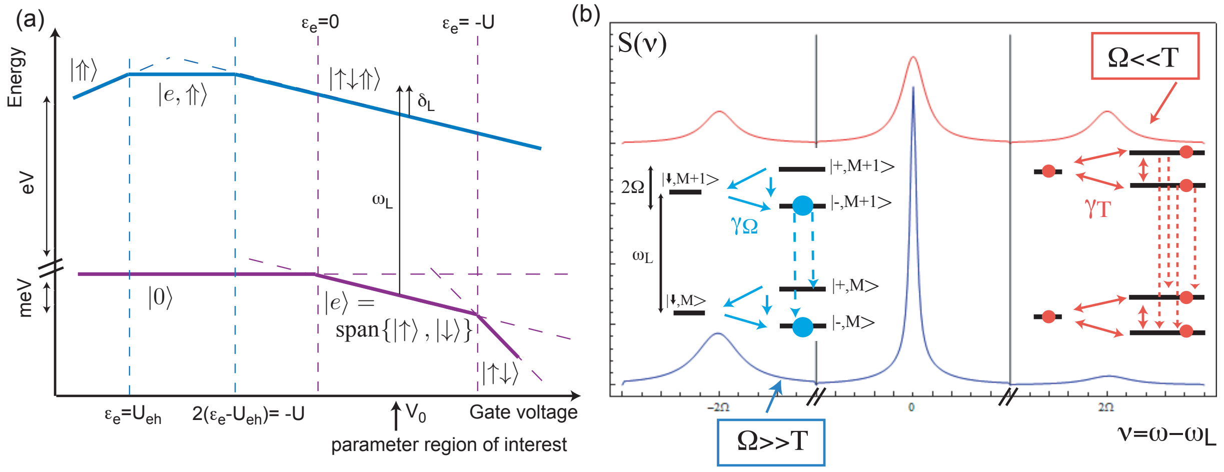


Figure S1: (a) Energy level diagram for $H_{QD}$ vs. gate voltage. We assume that the gate voltage is tuned to the vicinity of $V_0$ where the ground state of $H_{QD}|_{n_h=0}$ and $H_{QD}|_{n_h=1}$ carries one negative charge, $\omega_L$ is the laser frequency and $\delta_L$ the detuning from the bare QD-transition. (b) Application of a resonant laser ($\delta_L = 0$) and weak coupling to a FB at temperature $T \gg T_K$ leads to formation of QD dressed states $|\pm\rangle = (|\uparrow\downarrow\Uparrow\rangle \pm |\uparrow\rangle)/\sqrt{2}$ where $|\uparrow\rangle$ and $|\downarrow\rangle$ denote QD states carrying one electron of spin up or down, respectively, while $|\uparrow\downarrow\Uparrow\rangle$ denotes a negatively charged exciton including a hole. The index $M$ or $M-1$ counts the number of excitations (i.e. laser photons + holes), see [3], Ch. VI. Intra-manifold rates induced by the FB are denoted by solid arrows, steady state population by filled circles and spontaneous emission transitions by dashed arrows. The RF spectrum calculated using a Markovian master equation (neglecting Kondo correlations) shows a broadened Mollow triplet for $T_K \ll \Omega \ll T$ (red) and an asymmetric doublet for $\Omega \gg T \gg T_K$ (blue).

## NRG energy flow diagrams for the Rabi-Kondo model $H$

The numerical renormalization group (NRG) is a method to approximately diagonalize quantum impurity Hamiltonians where a few-level system, described by $H_{imp}$ (the impurity - or, in modern literature, the QD) is coupled to a (fermionic) bath, $H = H_{imp} + H_{imp-FB} + H_{FB}$ [4]. The strategy is to approximate $H_{FB}$ by

a tight-binding (Wilson-)chain where the coupling between two successive sites is exponentially decreasing as $\Lambda^{-n/2}$ for site index $n$, where $\Lambda > 1$ is a non-physical NRG discretization parameter. The QD is included as a site with index zero, only coupled to the first FB Wilson site (QD plus first FB Wilson site will be called "odd" Wilson chain). Each Wilson site can be identified with an exponentially decreasing energy scale $\Lambda^{-n/2}$, or, by looking at the associated fermionic wavefunction, with an exponentially increasing spatial separation $\Lambda^{n/2}$ from the QD position.

Due to the separation of energy scales along the Wilson chain, the chain Hamiltonian $H_N$, restricted to the first $N$ sites, can be diagonalized iteratively. After multiplying $H_N$ by $\Lambda^{N/2}$, the lowest eigenenergies can be plotted vs. $N$ in an NRG energy flow diagram, thus showing high to low energy scales of $H$ from left to right. Moreover, as a Wilson site can also be identified with a length scale in the impurity problem, the NRG flow accesses physics at increasing spatial separation from the impurity site with increasing $N$. Regions in which the rescaled eigenenergies form parallel horizontal lines are called fixed points - they can be described by fixed point Hamiltonians which are invariant under the renormalization group transformation.

Compared to computations of the quench spectral function in Ref. [5] for $\Omega = 0$, there are considerable conceptual changes for the computation in the $\Omega > 0$ case, described by the Rabi-Kondo model Hamiltonian, written as

$$H = \begin{pmatrix} H_{\mathrm{T}} & \Omega e_{\downarrow}^{\dagger} h_{\Uparrow}^{\dagger} \\ \Omega h_{\Uparrow} e_{\downarrow} & H_{\mathrm{K}} \end{pmatrix}. \tag{S3}$$

Most important is the loss of a quench setup between initial and final Hamiltonian, meaning that the hole is to be treated as a dynamic quantity. The NRG calculation in [5] relied on two separate NRG runs, separately diagonalizing the initial and final Hamiltonian given by $H_{\mathrm{K}} \equiv P_{\mathrm{K}} H P_{\mathrm{K}}$ and $H_{\mathrm{T}} \equiv P_T H P_T$, respectively. Then the corresponding two sets of eigenstates and -energies entered the analogue of Eq. (2). For $\Omega > 0$, however, we have to use only *one* NRG run for the full Hamiltonian $H$. Since this technical change comes with a number of important consequences, we first discuss these issues in the simple $\Omega = 0$ case.

For $\Omega = 0$, we define the ground state energy difference between $H_{\mathrm{T}}$ and $H_{\mathrm{K}}$ as

$$\Delta E \equiv E_{0,\mathrm{T}} - E_{0,\mathrm{K}} \tag{S4}$$

which has two contributions: On the one hand, the laser detuning $\delta_{\mathrm{L}}$ from the bare QD transition affects $\Delta E$ trivially, on the other hand, a hybridization $\Gamma > 0$ causes Kondo correlations in the $H_{\mathrm{K}}$ Kondo singlet ground state $|\mathrm{K}\rangle$ that additionally lower its energy. The energy level diagram is shown in Fig. S2(a) for $\Delta E > 0$ (laser tuned to bare QD transition, $\delta_{\mathrm{L}} = 0$) and $\Delta E = 0$ (b). Note that with a single logarithmic discretization, only low-lying eigenstates close to the overall ground state energy are resolved with increasing accuracy (orange rungs in Fig. S2 are NRG energy eigenvalues). This means if we use for example $\delta_{\mathrm{L}} = 0$ ($\Delta E > 0$), as shown in (a), the state $|\mathrm{K}\rangle$ is well resolved while the $|\mathrm{T}\rangle$ state is not well described in NRG and does not have a reasonable steady state population since $\rho_{\mathrm{ss}} \propto e^{-H/T}$. Numerically feasible is the case shown in (b). Using a laser blue-detuned with respect to the bare QD transition ($\delta_{\mathrm{L}} > 0$), one can counteract the correlation energy and push the $|\mathrm{K}\rangle$ up (relative to $|\mathrm{T}\rangle$) to

adjust $\Delta E = 0$. This leads to good resolution and finite population for both ladders, as the steady state expectation values $\langle P_{\mathrm{K}} \rangle \simeq 0.5 \simeq \langle P_{\mathrm{T}} \rangle$ show.

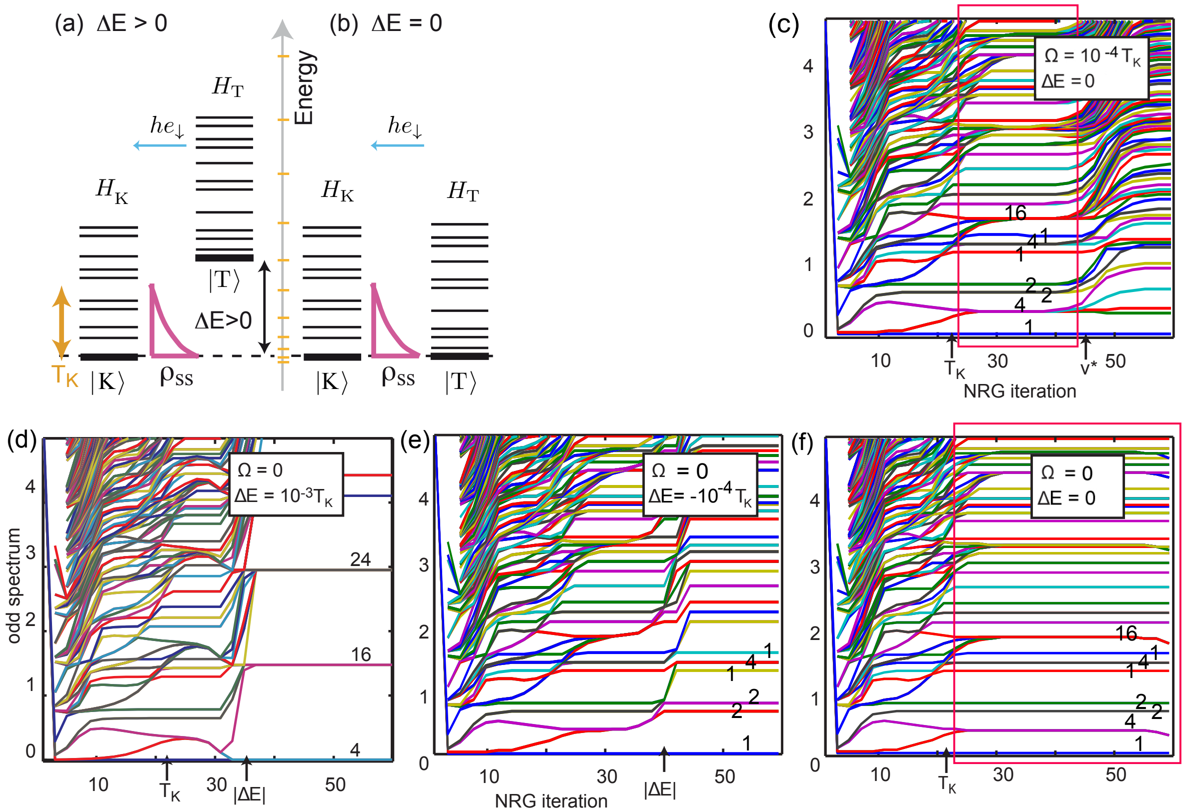


Figure S2: Effect of $\Delta E$ for one NRG diagonalization in the $\Omega = 0$ case: (a) $\Delta E > 0$ features a good resolution for the highly-correlated low-energy states above $|\mathrm{K}\rangle$, but not for the trionic states above $|\mathrm{T}\rangle$ and there is only a very small steady state hole population. (b) For $\Delta E = 0$, a good resolution for both families of states is achieved along with approximately equal steady state population in both ladders. (c) to (f): Flow diagrams for various parameter combinations $\Delta E$ and $\Omega$, with the red box showing the intermediate fixed point $H|_{\Omega=0}$. The NRG parameters are: Discretization $\Lambda = 2.7$, number of kept states $N_{\mathrm{keep}} = 1800$ and chain length $N_{\mathrm{max}} = 60$. The model parameters are the same as in Fig. 2 in the main text and the numbers attached to the final fixed point levels denote the degeneracies of the respective eigenenergies.

To find the right laser energy to compensate the ground state energy difference and ensure $\Delta E = 0$, NRG flow diagrams are employed: Both Hamiltonians $H_{\mathrm{T}}$ and $H_{\mathrm{K}}$ have distinct and well understood low energy fixed points: The $H_{\mathrm{K}}$ fixed point [obtained by setting $\Delta E > 0$ and $\Omega = 0$, see Fig. S2 (d)] describes the primary Kondo singlet state and its excitations. The degeneracies for odd Wilson site indices $n$ ('odd spectrum') are 4, 16,... . The $H_{\mathrm{T}}$ fixed point, describing the trion state and its excitations [$\Delta E < 0$ and $\Omega = 0$, see Fig. S2 (e)] features the degeneracies 1, 2, 2, 1, 4, 1,... . Consequently, since we still consider the uncoupled $\Omega = 0$ case, the $H$ flow diagram for $\Delta E = 0$ [Fig. S2 (f)] consists of a combination of the flow diagrams of the two decoupled Hamiltonians $H_{\mathrm{T}}$ and $H_{\mathrm{K}}$. This can be seen in detail by comparing state degeneracies (1, 4, 2, 2, 1, 4, 1, 16,...) which are a combination of the aforementioned degeneracies of $H_{\mathrm{K}}$ and $H_{\mathrm{T}}$. We used this fact as a technical trick guiding us how $\delta_{\mathrm{L}}$ should be fine-tuned to reach $\Delta E = 0$.

We now turn to the case where the trion and photon subspaces are coupled by stimulated absorption

and emission events for $\Omega > 0$. The parameter $\Delta E$ is still defined with respect to the $\Omega = 0$ case. Due to the discretization issues mentioned above, results for $|\Delta E| \gg \Omega$ should be regarded with care. We diagonalize the full Rabi-Kondo model, Eq. (S3). The flow diagram for $\Omega = 10^{-4} T_{\mathrm{K}}$ and $\Delta E = 0$ is shown in Fig. S2(c). We observe the emergence of a new fixed point below an energy scale

$$\nu^* \simeq \max\left(|\Delta E|, \Omega^*\right) \tag{S5}$$

which generalizes $\Omega^*$ from Eq. (5) for finite $\Delta E$.

Between the scales $T_{\mathrm{K}}$ and $\nu^*$, the fixed point spectrum for $\Omega > 0$ in Fig. S2 (c) has the same structure as the fixed point found for $\Omega = 0$ in Fig. S2 (f), as can be seen by comparison of the red boxes. Hence, the intermediate fixed point for $\Omega > 0$ in Fig. S2 (c) can be understood as a combination of $H_{\mathrm{K}}$ and $H_{\mathrm{T}}$. This further implies that the QD-perturbation $\Omega$, though local, only affects the system far away from the QD.

Eq. (S5) can be understood by noting that for finite $\Delta E^{(\prime)}$ the RG flow, Eq. (4), is augmented by a similar equation for $\Delta E'$ which, like the displaced charges, scales with $\Delta E'/D'$ and $\Omega'/D'$ in second order. Since $\Delta E'/D'$ and $\Omega'/D'$ are small initially compared to unity, $\Delta E'$ and $U'_\sigma$ do not flow appreciably under RG. Consequently, in the RG flow, the normalized TLS parameters $\Omega'/D'$ and $\Delta E'/D'$ increase. As soon as the larger one reaches unity, the scaling equations lose validity. For $|\Delta E'| \ll \Omega^*$, the renormalized Rabi frequency $\Omega'$ will increase to the renormalized bandwidth $D'$ before $D'$ reaches $\Delta E'$ and we enter the strong-$\Omega$ fixed point below $\Omega^*$, as discussed in the main text. If however $|\Delta E'| \gg \Omega^*$, the TLS energy splitting $\Delta E'$ determines the scale of the uncoupled fixed point, as expressed in Eq. (S5), for the unprimed parameters of the original model $H$.

The effect of Eq. (S5) on the broad peak position $|\nu_{\max}|$ of the emission spectrum is shown in Fig. S3(a). Analogously, the expression for the weight of the $\delta$-peak is also modified with a cutoff at $|\Delta E| = \Omega^*$ (Fig. S3(b)). For $|\Delta E| \gg \Omega^*$ the ground state contains either the trion or the Kondo state, so that $\delta_{\text{weight}} = |\langle h_\Uparrow e_\downarrow \rangle|^2$ vanishes due to AO between ground and post-quench state.

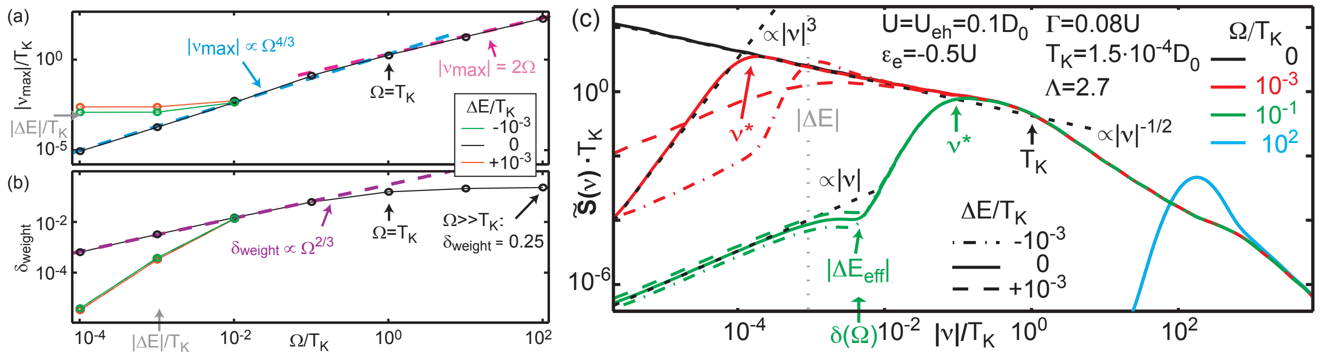


Figure S3: NRG results for the Rabi-Kondo model, Eq. (1), for finite $\Delta E$: The position of broad peak $|\nu_{\max}|$ in (a) and the weight of $\delta-$peak in (b) both deviate from the $\Delta E = 0$ case at $\Omega^* \simeq \Delta E$ where the nature of the low energy fixed point changes according to Eq. (S5). (c) Log-log plot of the normalized broad emission peak ($\tilde{S}\,(\nu < 0)$, for details on the normalization see below) for various parameters $\Omega$ and $\Delta E$. Thick solid lines denote spectra with $\Delta E = 0$, dashed and dash-dotted lines represent $\Delta E = \pm 10^{-3} T_{\mathrm{K}}$, respectively. The straight dashed lines represent power-law functions.

**Quantum Quenches and Beyond: Anderson Orthogonality, Hopfield Rule and their application for $S(\nu)$**

In this section, we provide some background information on the concept of Anderson Orthogonality (AO), the Hopfield Rule and their application in the discussion of the emission spectrum $S(\nu)$. The basic idea is that for $\Omega = 0$ spontaneous emission can be thought of as a transition corresponding to a quantum quench, showing AO, while for $\Omega \neq 0$, the signatures of AO are cut off at sufficiently low frequencies.

*Anderson Orthogonality (AO) and Hopfield Rule* (see also Ref. [6] for an extensive discussion): Whenever a quantum quench changes the local scattering potential for a FB, the overlap between the initial and final FB ground states, $|G_{\mathrm{i}}\rangle$ and $|G_{\mathrm{f}}\rangle$, vanishes with increasing electron number $N$ as $|\langle G_{\mathrm{i}}|G_{\mathrm{f}}\rangle| \propto N^{-\frac{1}{2}\Delta^2_{\mathrm{AO}}}$ where $\Delta_{\mathrm{AO}}$ is called the AO exponent. In the thermodynamic limit $N \to \infty$, the initial and final ground states are thus orthogonal for $\Delta_{\mathrm{AO}} \neq 0$. There are two important remarks: (i) Anderson [7] showed that the exponent $\Delta_{\mathrm{AO}}$ equals the displaced electronic charge (in units of $e$) in the quench, i.e.

$$\Delta_{\mathrm{AO}} = \langle G_{\mathrm{f}}|n_{\mathrm{tot}}|G_{\mathrm{f}}\rangle - \langle G_{\mathrm{i}}|n_{\mathrm{tot}}|G_{\mathrm{i}}\rangle \,, \tag{S6}$$

where $n_{\mathrm{tot}}$ counts the (spinless) electrons in a large volume $V_{\mathrm{large}}$ including the scattering site (QD). For spinful fermions, if the spin-channels are decoupled such that the FB ground states factorize, the correspondence is generalized to

$$\Delta^2_{\mathrm{AO}} = \Delta^2_{\mathrm{AO},\downarrow} + \Delta^2_{\mathrm{AO},\uparrow}. \tag{S7}$$

Note that by Friedel's sum rule, the displaced charge is connected to the scattering phase shift $\delta_\sigma$ for electrons with spin $\sigma = \pm$ by $\Delta_{\mathrm{AO},\sigma} = \delta_\sigma/\pi$. (ii) AO has important consequences for the low frequency behavior of generic quench spectral functions $\mathcal{A}$ similar to $S(\nu)$ in Eq. (2). AO causes the spectral function to behave as $\mathcal{A}(\nu) \propto \nu^{-1+\Delta^2_{\mathrm{AO}}}$, where $\nu$ is measured with respect to a threshold frequency.

*Application of AO to emission spectrum $S(\nu)$:* We start our discussion with the quench Hamiltonian $H|_{\Omega=0} = H_{\mathrm{QD,L}} + H_{\mathrm{QD-FB}} + H_{\mathrm{FB}} = H_{\mathrm{K}} + H_{\mathrm{T}}$ which we represent schematically in Fig. S4(a). The dashed line between the QD (circle) and the FB (box, in Wilson chain approximation) represents a tunnel coupling, the horizontal axis denotes decreasing energy or increasing length scales as in a NRG flow diagram (see above). If we assume $\Delta E = 0$, the degenerate ground state $|G\rangle|_{\Omega=0}$ is a superposition of the trionic state $|\mathrm{T}\rangle$, ground state of $H_{\mathrm{T}}$ shown in (b), and the Kondo singlet state $|\mathrm{K}\rangle = (|\uparrow\rangle|\mathrm{FB}_\downarrow\rangle - |\downarrow\rangle|\mathrm{FB}_\uparrow\rangle)/\sqrt{2}$, ground state of $H_{\mathrm{K}}$, depicted in (c). While $|\mathrm{K}\rangle$ features strong correlations between QD and FB, the trion state can be well approximated as a simple QD-FB product state $|\mathrm{T}\rangle = |\uparrow\downarrow\Uparrow\rangle|\mathrm{FB}_0\rangle$ where $|\mathrm{FB}_0\rangle$ is the unperturbed Fermi sea, i.e. all Wilson sites are half occupied. Let us take the state $|\mathrm{K}\rangle$ as reference, where the QD valence levels are filled (no holes present) and its conduction levels harbor half an electron of each spin. The region where the FB parts of the $|\mathrm{K}\rangle$ state, $|\mathrm{FB}_\sigma\rangle$, support an additional spin $\sigma$ (the screening cloud) is encircled by a yellow ellipse. Relative to $|\mathrm{K}\rangle$, the state $|\mathrm{T}\rangle$ features displaced charges $\Delta_{\mathrm{T},\sigma} = \sigma/2$, respectively (the $\Uparrow$-hole counts like a missing $\downarrow$-electron). Before discussing emission, let us consider an absorption event. Acting on $|G\rangle|_{\Omega=0}$ with the operator $e^\dagger_\downarrow h^\dagger_\Uparrow$, we first project on the component $|\mathrm{K}\rangle$ and then create a hole and a spin down electron in the conduction level. The resulting state can "lower its energy" [8] by adjusting its spin configuration to the $|\mathrm{T}\rangle$ state (b).

A priori, it is not obvious how an absorption process described by the operator $e^\dagger_\downarrow h^\dagger_\Uparrow$ for Hamiltonian

$H$ can be treated in the framework of AO. First, we recall a non-trivial feature of the Anderson impurity model underlying $H_{\rm K}$, namely that the low-energy fixed point below $T_{\rm K}$ can be described by potential scattering off the complicated Kondo screening cloud structure [5]. This observation implies that AO plays a role only for $|\nu| < T_{\rm K}$, as documented by an $-1/2$ power-law tail [5] which is explained as follows: Comparing the final state $|{\rm T}\rangle$, to the initial state $|{\rm K}\rangle$, the displaced charges (Eq. (S6)) read $\Delta_\sigma \equiv \Delta_{{\rm T},\sigma} - \Delta_{{\rm K},\sigma} = \sigma/2$. Consequently, for the quench connecting these two ground states in the long time limit, we find from Eq. (S7)

$$\Delta^2_{\rm AO} = \Delta^2_{{\rm AO},\downarrow} + \Delta^2_{{\rm AO},\uparrow} = (\Delta_{{\rm T},\uparrow} - \Delta_{{\rm K},\uparrow})^2 + (\Delta_{{\rm T},\downarrow} - \Delta_{{\rm K},\downarrow})^2 = 0.5. \tag{S8}$$

Since only the magnitude of the displaced charges, $(\Delta_{{\rm T},\sigma} - \Delta_{{\rm K},\sigma})^2$, enters this equation, $\Delta^2_{\rm AO}$ and the $-1/2$ power-law tail is the same for the emission process.

The second issue is the presence of the coherent laser drive, $H_{\rm QD-L} \propto \Omega$ in $H$ leading to stimulated absorption and emission processes. Thus spontaneous emission or absorption does *not* introduce a quantum quench, since the subspaces $P_{\rm T}$ and $P_{\rm K}$ are not dynamically decoupled [9]. However, if $\Omega$ is small, we can expect that the post-emission dynamics is not affected by the existence of $\Omega$ up to some time $\tau = 1/\Omega^*$ (i.e. $e^{i\tau H}(h_\Uparrow e_\downarrow)^\dagger e^{-i\tau H} \simeq e^{i\tau H|_{\Omega=0}}(h_\Uparrow e_\downarrow)^\dagger e^{-i\tau H|_{\Omega=0}}$ in Eq. (S1) for $\tau < 1/\Omega^*$) and that the spectral function therefore shows AO behavior as in a proper quench situation for $|\nu| > \Omega^*$. The relation between $\Omega^*$, $\Omega$ and the displaced charges can be found by a renormalization group analysis as sketched in the main text.

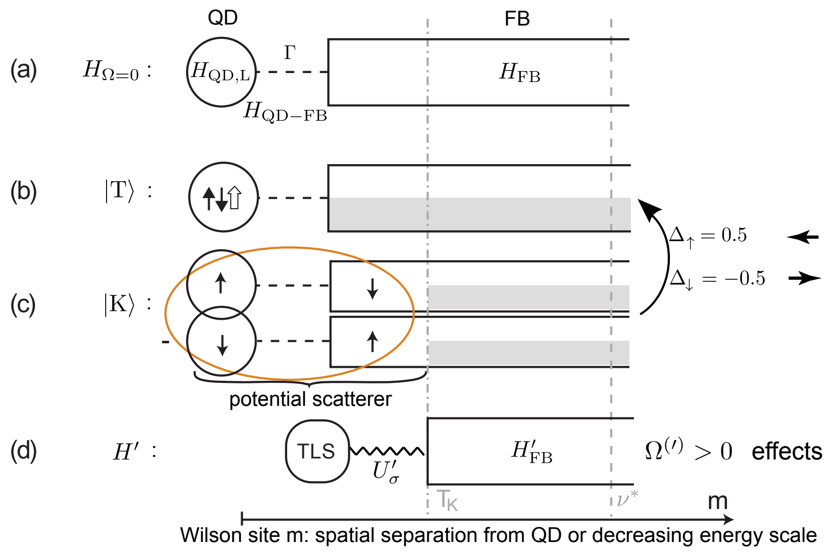


Figure S4: Cartoon of some Hamiltonians and states mentioned in the main text. (a) The quench Hamiltonian $H|_{\Omega=0}$ is of quantum impurity type, featuring a local QD and laser part tunnel coupled to the extended FB. The trionic state (b) can lower its energy after a spontaneous emission process mediated by $h_\Uparrow e_\downarrow$ by the formation of correlations (c) between QD and surplus FB spins where the latter are contained in a region of extent $1/T_{\rm K}$ around the QD (yellow ellipse). The Kondo singlet and trion configuration both act as potential scatterers for the surrounding FB electrons. The effective Hamiltonian $H'$, which explicitly contains a potential scattering term $\propto U'_\sigma$ in the trion sector, reproduces the respective scattering phase shifts of (b) and (c). In any case, effects due to $\Omega > 0$ are relevant above length scales $1/\nu^*$.

**Effective model $H'$**

Considering the NRG energy flow diagrams of the Rabi-Kondo model $H$ in Fig. S2 we noticed that the intermediate fixed point spectrum above $\nu^*$ is composed simply of a combination of the spectra of $H_{\rm K}$ and $H_{\rm T}$. This shows that in this intermediate energy range, the spectrum of the full Hamiltonian space can be decomposed into a direct sum of two subspectra, one describing the primary Kondo singlet state and its excitations, the other the trion and its excitations. These get coupled only at energy scales below $\nu^*$. This fact is the main motivation for constructing the effective Hamiltonian $H'$.

Before comparing $H$ and $H'$ NRG energy flow diagrams, we augment the heuristic derivation of the effective model $H'$ given in the main text in Eq. (3) by an intuitive graphical explanation in Fig. S4. The effective model $H'$ denoted schematically in Fig. S4(d) is designed to describe the effect of the transition between $|{\rm T}\rangle$ and $|{\rm K}\rangle$ [from (b) to (c)] on FB electrons beyond a separation $1/T_{\rm K}$ from the QD. The two-level-system (TLS), representing the QD plus the FB up to distance $1/T_{\rm K}$, controls the scattering potential $U'_\sigma$ [wavy line in (d)] for the surrounding FB electrons. If the TLS changes its state, so does the scattering potential – not only after a time scale $1/T_{\rm K}$ but (within the approximation of replacing $H$ by $H'$) instantaneously like in a X-ray absorption process. For $\Omega' = 0$, $\sigma'_z$ is conserved and the displaced electronic charge in a transition from $|{\rm K}\rangle_r$ to $|{\rm T}\rangle_r$ (TLS raising operators) is $\Delta'_\sigma = -1/\pi \cdot \arctan\left(\pi\rho' U'_\sigma\right)$ (in units of $e$, e.g. [6]). To reproduce the displaced charge $\Delta_\sigma = \sigma/2$ as found above, we require $\rho' U'_\sigma$ being equal to $-\sigma$ times a numerical value large compared to unity (we take $\rho' U'_\sigma = -50 \times \sigma$).

Now we can also consider the coherent QD-laser coupling. It is not a priori clear that $H'$ as given in Eq. (3), and the reasoning laid out above, would still be applicable for $\Omega^{(\prime)} > 0$. However, our NRG calculations show (in accordance with a renormalization analysis and the discussion below Eq. (S5)) that the $H|_{\Omega>0}$ flow diagram does not differ from the $\Omega = 0$ case for energies higher than $\nu^*$ (compare Figs. S2(c) and (f)), implying that it is indeed valid to consider the development of potential scattering and the effects of $\Omega$ *separately* as long as $\nu^* \ll T_{\rm K}$.

*NRG energy flow comparison for $H$ and $H'$:* One of the implicit assumptions in replacing $H$ by the effective Hamiltonian $H'$ with the scattering phase shifts as given above is that $n_{{\rm e}\uparrow} + n_{{\rm e}\downarrow} - n_{\rm h}$ exactly equals one. With the physical parameters as in Fig. 2 in the main text, this is only approximately true due to $U_{\rm eh} < \infty$. Although this small deviation has no observable consequences in the emission spectrum, turning to NRG energy flow diagrams resolving minute details of eigenstates and -energies, this issue will matter. Therefore, as an intermediate step for a flow diagram bases comparison of $H$ and $H'$, in Fig. S5 (a)-(c) we show the (odd) flow diagrams for $H|_{U_{\rm eh}=100D_0}$ where, as compared to the original $H$ spectra in Fig. S2, certain degeneracies in the trionic sector are restored. These flow diagrams then indeed agree with those for the effective model $H'$ [panels (d)-(f)].

**Discussion of emission spectra for $H^{(\prime)}$ in the case $\Delta E^{(\prime)} \neq 0$**

In Fig. S3(c), the Rabi-Kondo model emission spectrum, shown in Fig. 2(b,c) of the main text, is repeated for finite $\Delta E$. Since the total spectral weight is given by $\langle n_{\rm h} n_{{\rm e}\downarrow}\rangle \simeq O\left(\langle n_{\rm h}\rangle\right)$, it is strongly dependent on $\Delta E$. To enable mutual comparison between results for different values of $\Delta E$ we normalize all NRG spectra in this Supplemental Material as $\tilde{S}\left(\nu\right) \equiv S\left(\nu\right) / \langle n_{\rm h}\rangle$. Fig. S6(a) schematically summarizes the

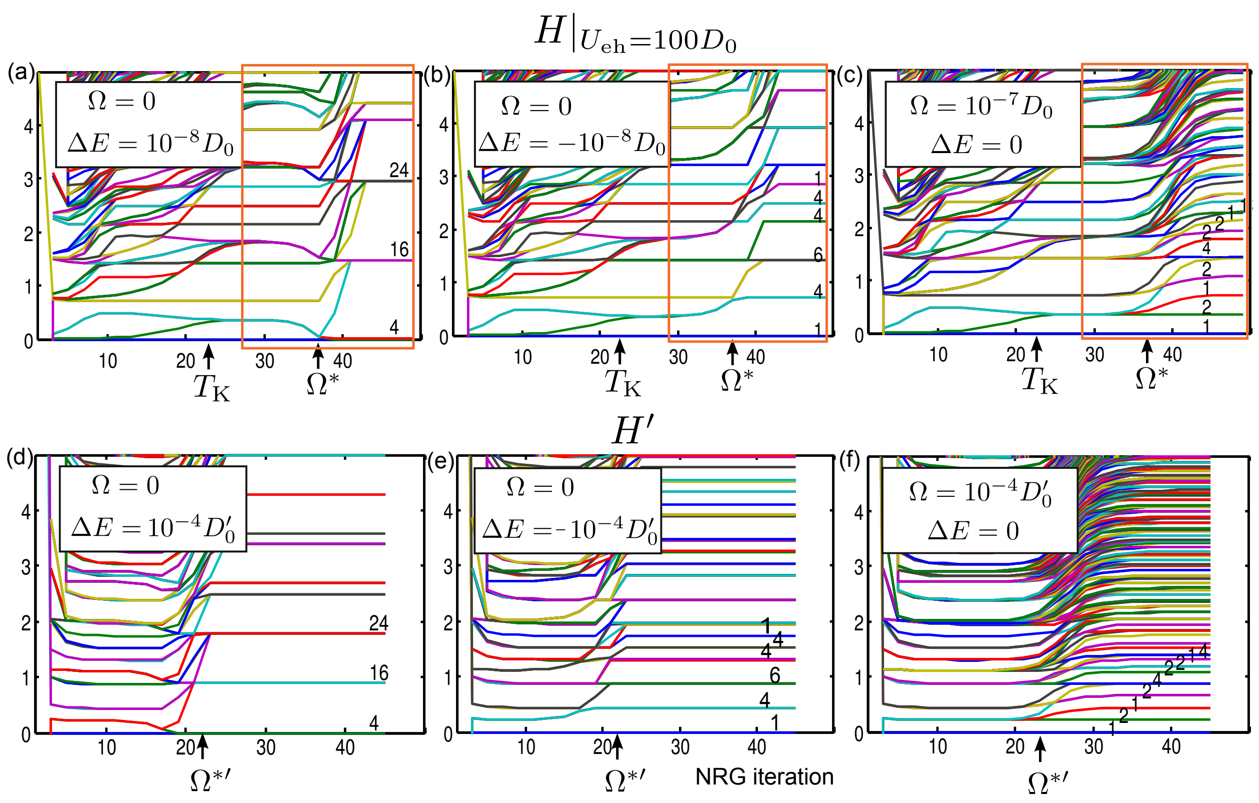


Figure S5: Comparison of NRG energy flow diagrams for $H|_{U_{\rm eh}=100D_0}$ [panels (a)-(c)] and $H'$ [panels (d)-(f)] for $\Delta E^{(\prime)} \lessgtr 0$ and $\Omega^{(\prime)} > 0$. With the QD/TLS defined as Wilson site zero, the $H|_{U_{\rm eh}=100D_0}$ flow diagrams show odd NRG iterations and the $H'$ diagrams even iterations such that an odd number of Wilson sites has been integrated out in going from $H$ to $H'$. The $H'$ flow diagrams mimic those of portions [boxed] of the $H|_{U_{\rm eh}=100D_0}$ flow diagrams that show the crossover from the intermediate to the strong-coupling fixed point.

generic features of the line shape. Coming from large detunings $|\nu|$, the characteristic power-law tails with exponents $-2$ (in the free orbital (FO) regime), $-1$ (in the local moment (LM) regime) and $-1/2$ (in the strong coupling (SC) regime), found and discussed by Türeci *et al.* in Ref. [5], are present also for $\nu^* < T_{\rm K}$. Curly brackets indicate the range of validity of several Hamiltonians mentioned in the main text. While treating $\Omega$ perturbatively using the quench Hamiltonian $H|_{\Omega=0}$ is a valid approximation for $|\nu| > \nu^*$, the effective Hamiltonian in Eq. (3) provides the appropriate approximate description for $|\nu| < T_{\rm K}$ and can explain the emergence of the low energy fixed point below $\nu^*$. The RF spectrum for the effective Hamiltonian $H'$, calculated using Eq. (2) but with $H'$ and $\sigma'_-$ taking the place of $H$ and $h_{\Uparrow}e_{\downarrow}$, respectively, is shown in Fig. S7. It indeed correctly reproduces all features of the $H$ spectrum for $|\nu| < T_{\rm K}$, which we now discuss.

The fixed point at energy $\nu^*$ causes a cut-off of the emission line shape; the nature of the line shape below the cut-off energy depends on $\Delta E$ and $\Omega$. Fig. S6(b) explains this regime $0 < |\nu| < \nu^*$ in detail, where we find a combination of $+3$ and $+1$ power-law tails as indicated schematically. We consider the two cases $\Omega^* \lessgtr |\Delta E|$ separately.

(i) For $\Omega^* > |\Delta E|$, the transition between the $+3/+1$ power-law tails occurs at a scale

$$\Delta E_{\text{eff}} = \Delta E + \delta(\Omega) > \Delta E, \tag{S9}$$

where $\delta(\Omega)$ denotes an $\Omega$-dependent effective detuning with $0 < \delta(\Omega) \ll \Omega$ that captures the small driving dependence which is attributed to second-order effects in the RG equations for $\Delta E'$ discussed above. The $+3/+1$ crossover is either sharp for $\Delta E_{\text{eff}} > 0$ or gradual in the case $\Delta E_{\text{eff}} < 0$. The analysis for the $+1$ exponent parallels the discussion for the $+3$ exponent in terms of the secondary Kondo model $H'_{\text{K}}$ given in the main text: The presence of an effective magnetic field ($\Delta E_z \neq 0$) in Eq. (6), corresponding to a finite $\Delta E^{(\prime)}$ in models $H$ and $H'$, causes the density of the $z$-component of the spin in $H'_{\text{K}}$ to acquire a nonzero average. Hence, the correlation function $S'_z s'_z(0)$ will have components containing the correlator of just two Fermi operators with their conjugates, which decays as $t^{-2}$, leading to a $\sim |\nu|^{+1}$ behavior of the spectral function.

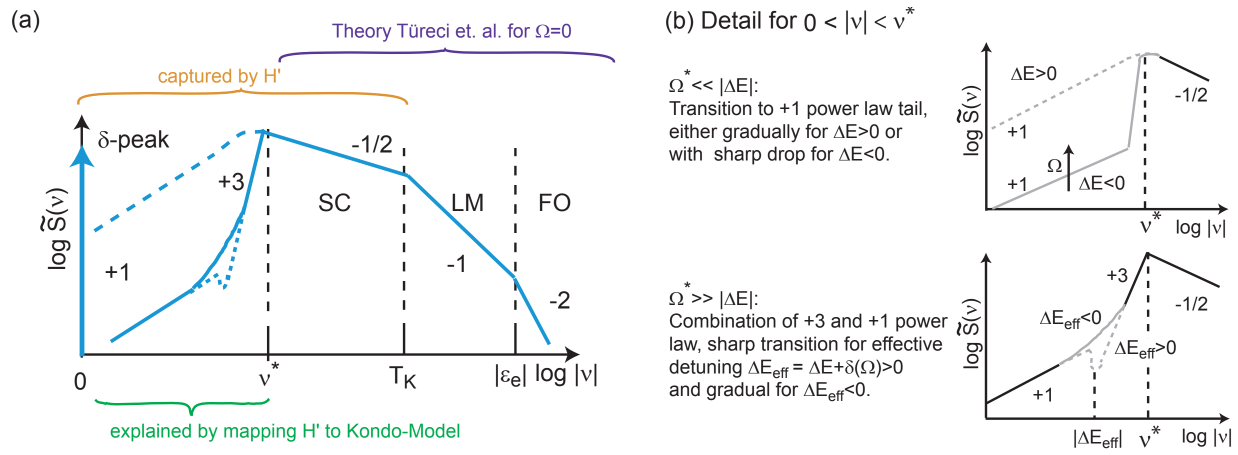


Figure S6: Phenomenological discussion of $\tilde{S}(\nu)$, revealing characteristic power-law tails. The same discussion applies to $\tilde{S}'(\nu)$ (for the effective Hamiltonian $H'$) for $|\nu| < T_{\text{K}}$.

The effect described in Eq. (S9) can be clearly seen in the $H$ spectrum for $\Delta E = 0$ (Fig. S3(c), $\Omega = 10^{-1}T_{\text{K}}$, green solid line) which shows a transition to a $+1$ tail at $\Delta E_{\text{eff}} = \Delta E + \delta(\Omega) = \delta(\Omega)$. Further, the $\Omega = 10^{-1}T_{\text{K}}$ spectra for $\Delta E = \pm 10^{-3}T_{\text{K}}$ (green dashed and dash-dotted lines) do not differ significantly since we have $\delta(\Omega) \gg \Delta E$ and thus, according to Eq. (S9), $\Delta E_{\text{eff}}$ is virtually equal in both cases.

(ii) Turning to $\Omega^* < |\Delta E|$, (dash and dashed-dotted red lines in Fig. S3(c)) the $+3$ tail is absent; in the case $\Delta E > 0$ a smooth transition to the $+1$ tail occurs while for $\Delta E < 0$ this transition is realized in a steep drop beyond NRG's smoothing resolution limit. This steep drop can be understood in the limiting case $\Omega \to 0$ as a horizontally displaced $\Omega = \Delta E = 0$ curve which has a threshold at $|\nu| = -\Delta E$.

## Implications for an experimental study and outlook

The NRG results shed light on the results of the competition between Kondo physics and the laser coupling. As expected, the ratio of $T_{\text{K}}$ and $\Omega$ determines the predominant form of the emission line shape, an asymmetric power-law-divergent peak in the Kondo-dominated regime $\Omega \ll T_{\text{K}}$, and a double

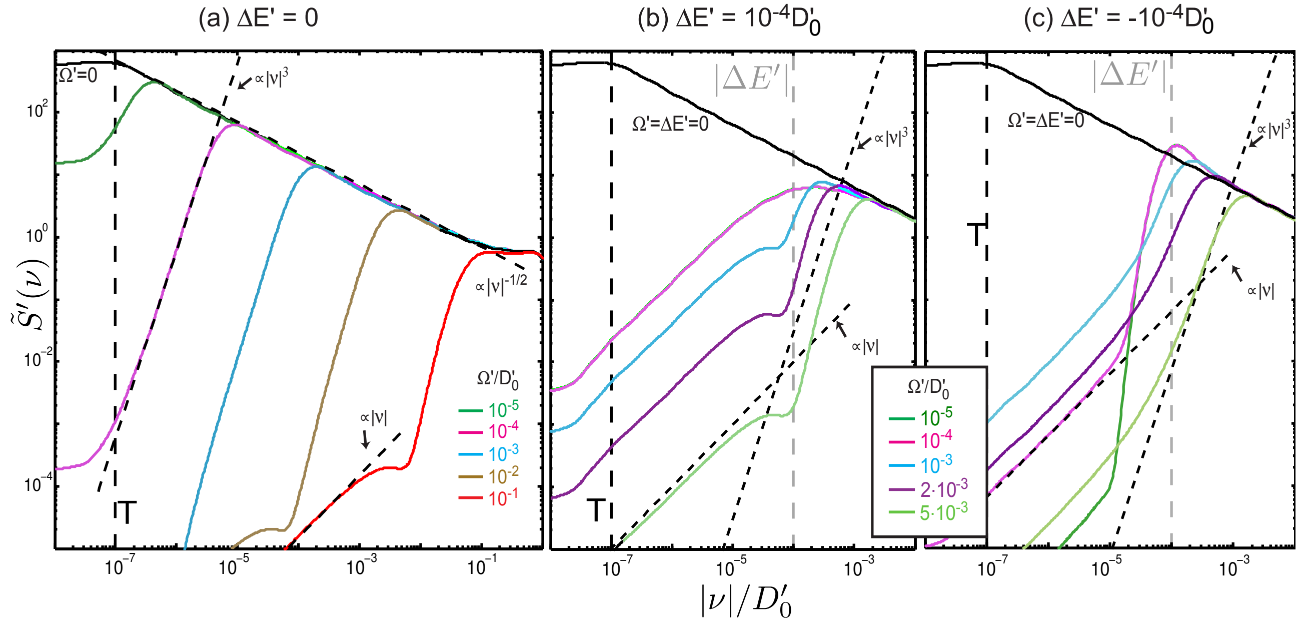


Figure S7: $\tilde{S}'(\nu<0)$ for $H'$ (without $\delta$−peak). (a) $\Delta E' = 0$, (b) $\Delta E' > 0$ and (c) $\Delta E' < 0$. For reference, the $\Omega' = \Delta E' = 0$ spectrum is repeated in all plots (solid black line).

peak structure in the limit $\Omega \gg T_{\mathrm{K}}$. However, the role of the seemingly weaker effect is interesting: A dominant driving laser leaves no trace of Kondo physics while dominant Kondo physics renormalizes $\Omega$ to a smaller value but preserves its characteristic non-trivial double peak feature in the spectrum. This explains our focus on the regime $\Omega < T_{\mathrm{K}}$, which is highly attractive for further experimental study. We remark that the main results should be also valid in a two laser setup (creating dressed states with one laser, probing absorption with another), which might be experimentally more feasible than standard resonance fluorescence.

For a strongly coupled device and temperatures $T \ll T_{\mathrm{K}}$, Kondo signatures in the absorption line shape of a weak laser have already been detected in experiment [10]. An order of magnitude separation between $T$ (which flattens out all spectra for $|\nu| \lesssim T$) and $T_{\mathrm{K}}$ as well as a spontaneous emission rate below $T$ has been achieved. For obtaining the predicted double peak structure in the resonance fluorescence experiment with $\Omega < T_{\mathrm{K}}$, the crucial condition $T \ll \nu^* \ll T_{\mathrm{K}}$ has to be fulfilled. We expect that a non-zero spontaneous emission rate will lead to partial broadening of the $\delta$-peak at zero detuning, separating into an elastic and inelastic component. For the proper inclusion of spontaneous emission in the theoretical treatment, we propose an extension of the current study using the framework of Lindblad-NRG, currently under development [11].

The total area of the peak at the laser frequency and the peak-to-peak separation to the red emission peak are predicted to scale with $\Omega$ to the power 2/3 and 4/3, respectively. This is valid if $\Delta E$ (controlled by the laser detuning) is smaller than the renormalized Rabi frequency $\Omega^*$. Compared to the measurement of power-law tails as signatures of Kondo physics, which require experimental data with sufficiently low noise level, peak areas and peak-to-peak separations can be measured with relative ease. Further, the scaling collapse of the broad emission peak with respect to $\nu^*$, which is theoretically valid only for $S(\nu)$

with $|\Delta E_{\rm eff}| < |\nu| < T_{\rm K}$, should be a robust experimental feature since the regions where scaling fails (i.e. $|\nu| > T_{\rm K}$, $|\nu| < |\Delta E_{\rm eff}|$) are expected to support only a small spectral signal, effectively well below the noise level.

It is interesting to compare the effect of a laser drive $\Omega$ with the consequences of a nonzero magnetic field $B$ (which we have set to zero throughout this work). While a circularly polarized laser coupling in a QD removes the degeneracy of the spin up and down state just like a magnetic field $B$ does, their signatures in the emission spectrum in presence of Kondo physics are strikingly different. While a magnetic field $|B| < T_{\rm K}$ results in a smooth modification of the $B = \Omega = 0$ fixed point (and consequently changes the $-1/2$ power-law exponent in the RF line shape [5, 10]) a Rabi frequency $\Omega < T_{\rm K}$ induces a *new* low energy fixed point while keeping the power-law exponent at $-1/2$. For nonzero $B$ *and* $\Omega$ (both $< T_{\rm K}$) we conclude that a modification of the $\Omega$-scaling dimension $\eta_x$ (in the original Rabi-Kondo model) due to $B$ would modify the 4/3 and 2/3 exponents for the $\Omega^*$ and $\delta_{\rm weight}$-scaling with $\Omega$. Thus, application of a magnetic field could enhance the visibility of scaling effects on the emission spectrum in experiment.

## References


[1] B. Sbierski, A. Imamoglu. (to be published).

[2] H. Breuer, F. Petruccione, *The Theory of Open Quantum Systems* (Oxford, 2002).

[3] C. Cohen-Tannoudji, J. Dupont-Roc, G. Grynberg, *Atom-Photon Interactions* (Wiley, 1992).

[4] R. Bulla, T. A. Costi, T. Pruschke, *Rev. Mod. Phys.* **80**, 395 (2008).

[5] H. E. Türeci, *et al.*, *Phys. Rev. Lett.* **106**, 107402 (2011).

[6] W. Münder, A. Weichselbaum, M. Goldstein, Y. Gefen, J. von Delft, *Phys. Rev. B* **85**, 235104 (2012).

[7] P. W. Anderson, *Phys. Rev. Lett.* **18**, 1049 (1967).

[8] Of course, unitary evolution cannot change a state's energy and evolve the post quench state to the Kondo singlet state. More precisely, consider the overlap between post-emission state and its time-evolved version in Eq. (S1): Expanding in energy eigenstates, for times larger than $1/T_K$ the overlap has contributions only from strongly correlated eigenstates below energy $T_K$.

[9] However, spontaneous emission can be interpreted as a quench between two adjacent excitation manifolds in the dressed state picture of resonance fluorescence.

[10] C. Latta, *et al.*, *Nature* **474**, 627 (2011).

[11] I. Weymann, A. Weichselbaum, J. von Delft, *(to be published)* .
